# Supplementary material for: Equivariance Discovery by Learned Parameter-Sharing
Source: arXiv:2204.03640 source file (2022-04-07)
Supplement: Supplementary file 1 [file supp_partition_distance.tex]

\section{Partition Distance for Evaluation} \label{sec:supp_partition_distance}
We review the definition of the partition distance and discuss its relevance to evaluating the discovered equivariance. 
To formally define the partition distance, we first define what is a cluster and a partition, following~\citet{gusfield2002partition}.
\begin{definition}[Cluster]
Given a set $\gS$, a cluster is a non-empty subset of $\gS$, \ie, $\gC \subseteq \gS$ where $\gC \neq \emptyset$.  
\end{definition}

\begin{definition}[Partition]
A partition of $\gS$ is a set of clusters, $\gP_\gS = \{\gC_i\}$, where $\gC_j \cap \gC_k = \emptyset \;\;\forall j \neq k$ and $\bigcup_{i=1}^{|\gP_\gS|} \gC_i = \gS$. In other words, the elements in $\gS$ are ``partitioned'' into mutually exclusive sets.
\end{definition}

\begin{definition}[Partition Distance]
Given two partitions of a set, the partition distance is the number of elements that must be moved between the clusters such that the two partitions are identical.
\end{definition}

Next, consider the Gaussian with shared means problem in~\secref{sec:analyze} where we model the mean as
$$
\theta = \mA\phi.
$$
Here, $\bm\theta, \bm\psi \in \mathbb{R}^{K}$, $\mA \in \{0,1\}^{K \times K}$, and $\mA$ is row stochastic, \ie, $\sum_j \mA_{ij} = 1$. 

A parameter-sharing scheme $\mA$ can be viewed as a partition over the set of model parameters. As $\mA$ is integral row stochastic, %
it forms a partition of mutually exclusive clusters. Given two parameter-sharing schemes $\mA^{(1)}$ and $\mA^{(2)}$ the parition distance $PD(\mA^{(1)}, \mA^{(2)})$ can be efficiently computed, in polynomial time, as proposed by~\citet{gusfield2002partition}. We will next explain how this distance relates to equivariance. 

Given a sharing scheme $\mA^{(i)}$, we write it in the form of a partition
\bea
\gP_K^{(i)} = \{ \gC^{(i)}_k | \;\forall k \in [1\dots K]\} \text{ and } \gC^{(i)}_k = \{j  | \mA^{(i)}[j,k]==1\}.
\eea

Due to the shared parameters, the dimensions within a cluster can be permuted.
In other words, given $\mA^{(i)}$, the model is $\gG_{K,K}^{(i)}$-equivariant, where 
\be
\gG_{K,K}^{(i)} = \bigcup_{\gC^{(i)}_k \in \gP^{(i)}_k} \Pi_{\gC^{(i)}_k}.
\ee
We use $\Pi_{\gC^{(i)}_k}$ to denote the set of all possible permutation matrices over the dimensions in $\gC^{(i)}_k$, while holding the remaining dimensions fixed. 

We consider the symmetric difference of two sets for quantifying the similarity between $\gG$-equivariances, \ie, 
\be
\gG^{(1)} \Delta \gG^{(2)} = (\gG^{(1)} - \gG^{(2)}) \cup  (\gG^{(2)} - \gG^{(1)}).
\ee
This captures the non-overlapping elements within the groups. We now relate this quantity to the partition distance.

\vspace{0.2cm}
\begin{mdframed}[style=MyFrame]
\begin{claim}\label{clm:pd}
Consider the above Gaussian sharing setup. Then
\bea
\kappa \cdot  PD(\mA^{(1)}, \mA^{(2)}) \geq |\gG_{K,K}^{(1)} \Delta \gG_{K,K}^{(2)} | \geq PD(\mA^{(1)}, \mA^{(2)}),
\eea
where $\kappa = K!-1$ is a constant and $K$ is the number of dimensions.
\end{claim}
\end{mdframed}

We discuss the result's significance before presenting the proof. 
From~\clmref{clm:pd}'s upperbound, 
\be
PD(\mA_1, \mA_2)=0 \;\;\longrightarrow\;\; |\gG_{N,N}^{(1)} \Delta \gG_{N,N}^{(2)} |=0.
\ee 
Hence, when a partition distance is zero, the two sharing schemes achieve the same equivariance property. Next, as the symmetric difference is lower bounded by the partition distance, when the partition distance is non-zero, then the equivariance properties are not identical. Base on these properties and its efficiency to compute, we find partition distance to be a suitable evaluation metric.
\begin{proof} 
Let  $\gP_K^{(1)}$ and $\gP_K^{(2)}$ denote the corresponding partitions of $\mA^{(1)}$ and $\mA^{(2)}$. 

Let $j$  be an element that must be moved in $\gP_K^{(1)}$ to match $\gP_K^{(2)}$. 

Let $\gC_{j*}^{(1)}$ and $\gC_{j*}^{(2)}$ refer to the cluster that contains the element $j$. 

\textbf{Lower bound.} As $j$ must be moved, this means that $\gC_{j*}^{(1)}$ are $\gC_{j*}^{(2)}$ are not identical, therefore, $|\Pi_{\gC_{j*}^{(1)}} \;\Delta\; \Pi_{\gC_{j*}^{(2)}}| \geq 1$. 

As $\Pi_{\gC_{j*}^{(1)}}  \subseteq  \gG_{K,K}^{(1)} $ and $\Pi_{\gC_{j*}^{(2)}}  \subseteq  \gG_{K,K}^{(2)} $, \underline{for each $j$} there exist a difference of at least 1. Therefore, $$|\gG_{K,K}^{(1)} \Delta \gG_{K,K}^{(2)} | \geq PD(\mA^{(1)}, \mA^{(2)}).$$

\textbf{Upper bound.} Similarly,
we can upper bound $|\Pi_{\gC_{j*}^{(1)}} \;\Delta\; \Pi_{\gC_{j*}^{(2)}}|$ with $K!-1$. Consider the case, when $\gC_{j*}^{(1)}$ contains all the elements and $\gC_{j*}^{(2)}$ contains only $j$. 

As $\Pi_{\gC_{j*}^{(1)}}  \subseteq  \gG_{K,K}^{(1)} $ and $\Pi_{\gC_{j*}^{(2)}}  \subseteq  \gG_{K,K}^{(2)} $, \underline{for each $j$} there exist a difference of at most $K!-1$. Therefore, $$(K!-1)  \cdot PD(\mA^{(1)}, \mA^{(2)}) \geq \gG_{K,K}^{(1)} \Delta \gG_{K,K}.$$ Note, a tighter upper-bound can be derived. We provide this result for  ease of understanding.
\end{proof}
